# Supplementary material for: RAIL: Reachability-Aided Imitation Learning for Safe Policy Execution
Source: arXiv:2409.19190 source file (2024-09-28)
Supplement: Supplementary file 1 [file A_appendix.tex]

\section{Appendix}

\subsection{Safe Learning-based Control Benchmarks}
To establish the common ground for the safety-related literature, we list some prominent benchmarks \cite{Ray2019, yuan2022safe, zhao2023guard, leike2017ai, ji2023safety, Gronauer2022BulletSafetyGym}. 

The \textbf{Safety Gym} \cite{Ray2019} is a benchmark released by OpenAI for safe exploration with a special focus on evaluating the performance of constrained RL \textit{while training}.
The \textbf{Safe control gym} \cite{yuan2022safe} is a benchmark that supports Safe RL algorithms and safety-filter algorithms, using Pybullet.
The \textbf{GUARD} \cite{zhao2023guard} is a safe RL benchmark by Changliu's group that supports manipulators as an agent. Their code is beautiful.
The \textbf{Safety Gymnasium} \cite{ji2023safety} is also one of the most active gymnasiums that builds on the Mujoco engine.

What would be a good task, for a gymnasium to integrate diffusion-policy and safety-gym: would depend on the simulator it uses (Pybullet, Mujoco), agents, and tasks that it supports.

After this study, we hope to figure out 1) what example is mostly dealt with in Safe-RL literature, 2) hint on what would be the difference between safe-RL and safe-diffusion policy, and 3) any paragons of safe manipulation, 4) safe imitation learning, 5) if diffusion policy is currently limited to imitation learning, 6) can diffusion-policy be viewed as RL way.

\subsection{Notable Safe RL Algorithms}
This section reviews existing Safe RL algorithms. Given the infancy of diffusion policy, we expect that Safe Diffusion would be largely influenced by the Safe RL literature.
\begin{itemize}
    \item Safety Layer
    \item Recovery RL
\end{itemize}

\subsection{Approaches Overview (Idea)}
The motivation of this project is to design a \textit{safety filter} for the diffusion policy, meaning that it overrides the diffusion policy only when it is unsafe.
There exist three ways of solving this problem.

\begin{algorithm}[t]
\label{algo:simulate-parc-tree}
\small
\caption{Receding Horizon Safety Filter}
\DontPrintSemicolon
\label{algo:parc-tree}
\textbf{Input:} $x_0, g, \mathcal O$ \;
$done \gets False$ \;
$s_{bkup} \gets safePlan(x_0)$ \;
\While{not done}{
    $backup \gets False$ \;
    $s_{0..H} \gets \textbf{diffusionPolicy}(s_0; g, \mathcal O)$ // Algorithm A\; 
    $FO \gets \textbf{reach}(s_{0..1})$ // Algorithm B\; 
    \If{FO \cap ~ \mathcal O = \phi}{ 
        $k^* \gets \textbf{safetyLayer}(s_{1..H}; FO))$ // Algorithm C\; 
        \If{$k^*$ exists}{
            $s_{bkup} \gets (s_{0..1}, k^*)$ \;
            backup \gets True
        }
    }
     \eIf{backup}
     {$s_{next} \gets s_1$\;}
     {$s_{next} \gets s_{bkup}.pop()$\;}

     $a \gets control(s_0, s_{next})$\;
     $s_0 \gets simulate(s_0, a)$\;

     \If{s_0 == g}{
     $done \gets True$\;
     }
}
\end{algorithm}

\subsection{Manipulator Robots for Learning}

\begin{table*}[h]
\centering
\begin{tabular}{|l|l|l|l|}
\hline
\textbf{Methodology} & \textbf{Task Specification} & \textbf{Arm Manipulator} & \textbf{Reference} \\ \hline
\multicolumn{4}{|c|}{\textbf{Multi-agents}} \\ \hline
Diffusion Policy & Evader reaches target & Franka& \cite{chi2023diffusion} \\ \hline
Diffusion Policy & Evader reaches target & UR5 & \cite{chi2023diffusion} \\ \hline
Diffusion Policy & Evader reaches target & Kuka & \cite{chi2023diffusion} \\ \hline
Diffusion Policy & Evader reaches target & Kinova & \cite{chi2023diffusion} \\ \hline

\end{tabular}
\caption{Learning + Manipulator}
\label{table:systems_constraints_various}
\end{table*}

%%%%%%%%%%%%%%%%%%%%%%%%%%%%%%%%%%
%%%%%     Diffusion Policy  %%%%%%
%%%%%%%%%%%%%%%%%%%%%%%%%%%%%%%%%%
\begin{table*}[h]
\centering
\begin{tabular}{|l|l|l|l|}
\hline
\textbf{Methodology} & \textbf{Task Specification} & \textbf{Arm Manipulator} & \textbf{Reference} \\ \hline
\multicolumn{4}{|c|}{\textbf{Multi-agents}} \\ \hline
HJ + RL & Evader reaches target & No collision with chaser & \cite{hsu2021safety} \\ \hline

\end{tabular}
\caption{Diffusion Policy for Robotics}
\label{table:systems_constraints_various}
\end{table*}

\subsection{Zonotopes and Polynomial Zonotopes}
To enable reachability analysis and swept volume computation, we use zonotopes and polynomial zonotopes \cite{kochdumper2020sparse}.
Consider a center $\vc{c} \in \R^n$ and a \textit{generator matrix} $\Gen = [\gen_1,\cdots,\gen_m] \in \R^{n\times m}$ and a vector of \textit{indeterminates} $\ind$.
A zonotope is the set
\begin{align*}
    \set{Z} = \zonotope(\ctr,\Gen,\ind) = \Big\{
        \vc{z} \in \R^n \mid
        \vc{z} = \Gen\ind,\ \ind \in [-1,1]^m
    \Big\}.
\end{align*}

Additionally, consider an \textit{exponent matrix} $\xpn_i \in \N_m$.
A polynomial zonotope is the set
\begin{align*}
    \set{P} = \polyzono(\Gen,\Xpn,\ind) = \Big\{
        \vc{p} \in \R^n \mid
        \vc{p} = \sum_{i=0}^m \gen_i\ind^{\xpn_i},\ 
        \ind \in [-1,1]^m
    \Big\}.
\end{align*}
We perform addition, multiplication, and cross products on polynomial zonotopes.

\textit{Addition:}
Let $\set{P}_1 = \polyzono(\Gen_1,\Xpn_1,\ind_1)$ and $\set{P}_2 = \polyzono(\Gen_2,\Xpn_2,\ind_2)$ with $m_1$ and $m_2$ generators, respectively.
Their Minkowski sum is
\begin{align*}
    \set{P}_1 \oplus \set{P}_2 =
    \polyzono([\Gen_1,\Gen_2],\diag(\Xpn_1,\Xpn_2),[\ind_1;\ind_2]).
\end{align*}

\textit{Multiplication:}
Suppose $\set{P}_1 \subset \R^{n\times m}$ and $\set{P}_2 \in \R^{m\times k}$, meaning the generators are matrices.
Then their product is
\begin{align*}
    \set{P}_1\set{P}_2 = \left\{
        \vc{M} \in \R^{n\times k} \mid
        \vc{M} = \sum_{i=0}^{m_1}\gen_{1,i}\Big(
                \sum_{j=0}^{m_2}\gen_{2,j}\ind_2^{\xpn_{2,j}}
            \Big)\ind_1^{\xpn_{1,i}}
    \right\},
\end{align*}
where $\gen_{1,\star}$ and $\xpn_{1,\star}$ are from $\set{P}_1$, $\gen_{1,\star}$ and $\xpn_{1,\star}$ are from $\set{P}_2$.
Notice that $\set{P}_1\set{P}_2$ is again a polynomial zonotope (also see \cite{kochdumper2020sparse,michaux2023can}).

\textit{Cross Product:}
Suppose $\set{P}_1, \set{P}_2 \in \R^3$, and each \ith generator of $\set{P}_1$ is $\gen_i = [g_{i,1},g_{i,2},g_{i,3}]\trans$.
Define
\begin{align*}
    \set{P}_1^\times = \left\{
        \vc{M} \in \R^{3\times 3} \mid
        \vc{M} = \sum{i=0}^{m_1}
            \left[\begin{smallmatrix}
                0 & -g_{i,3} &* g_{i,2} \\
                g_{i,3} & 0 & -g_{i,1} \\
                -g_{i,2} & g_{i,1} & 0
            \end{smallmatrix}\right]
            \ind_1^{\xpn_{1,i}}
    \right\}.
\end{align*}
Then the set-based cross product is $\set{P}_1\otimes\set{P}_2 = \set{P}_1^\times\set{P}_2$.
